# Supplementary material for: Teacher Perception of Automatically Extracted Grammar Concepts for L2 Language Learning
Source: arXiv:2206.05154 source file (2022-06-10)
Supplement: Supplementary file 1 [file supplementary.tex]

\newpage
\appendix

\input{images/autolex-usability-questions}

\input{images/autolex-results}
